# Supplementary material for: Learning Real Facial Concepts for Independent Deepfake Detection
Source: arXiv:2505.04460 source file (2025-05-07)
Supplement: Supplementary file 1 [file X_suppl.tex]

\clearpage
\setcounter{page}{1}

\stepcounter{section} % 让section计数器增加1
\setcounter{section}{0} % 将section计数器重置为0
\setcounter{equation}{0}

\setcounter{figure}{0}

\setcounter{table}{0}

\setcounter{footnote}{0}
\maketitlesupplementary

\begin{figure}[h]
    \raggedright
    \includegraphics[width=0.25\linewidth]{sec/author_img/MinghuiLiu.jpg}
\end{figure}
Ming-Hui Liu is currently pursuing the Ph.D. degree in software engineering at the School of Software, Shandong University, Jinan, China. Her research interests include computer vision and she focuses on the subfields of deepfake detection and person re-identification.

\begin{figure}[h]
    \raggedright
    \includegraphics[width=0.25\linewidth]{sec/author_img/Harry_Cheng.jpg}
\end{figure}
{Harry Cheng} received the B.Eng. and master degree from Shandong University, China, in 2018 and 2021, respectively. He is currently pursuing the Ph.D. degree with the School of Computer Science and Technology, Shandong University, under the supervision of Liqiang Nie. His research interests include Deepfake detection and multi-modal computing.

\begin{figure}[h]
    \raggedright
    \includegraphics[width=0.25\linewidth]{sec/author_img/Tianyi_Wang.jpg}
\end{figure}
{Tian-Yi Wang} received the the double major B.S. degrees in Computer Science and Applied and Computational Mathematical Sciences from the University of Washington, Seattle, USA, in 2018. After that, he received the Ph.D. degree in Computer Science from The University of Hong Kong, Hong Kong, in 2023. He is currently a Research Fellow with Nanyang Technological University, Singapore. His major research interests include multimedia security and forensics, face forgery detection, and computer vision.

\vspace{20em}

\begin{figure}[h]
    \raggedright
    \includegraphics[width=0.25\linewidth]{sec/author_img/luoxin.png}
    \label{fig:enter-label}
\end{figure}
Xin Luo received the Ph.D. degree in computer science from Shandong University, Jinan, China, in 2019. He is currently an assistant professor with the School of Software, Shandong University, Jinan, China. His research interests mainly include machine learning, multimedia retrieval and computer vision. He has published over 20 papers on TIP, TKDE, ACM MM, SIGIR, WWW, IJCAI, et al. He serves as a Reviewer for ACM International Conference on Multimedia, International Joint Conference on Artificial Intelligence, AAAI Conference on Artificial Intelligence, the IEEE Transactions on Cybernetics, Pattern Recognition, and other prestigious conferences and journals.

\begin{figure}[h]
    \raggedright
    \includegraphics[width=0.25\linewidth]{sec/author_img/XInshun-xu.jpg}
\end{figure}
Xin-Shun Xu is currently a professor with the School of Software, Shandong University. He received his M.S. and Ph.D. degrees in computer science from Shandong University, China, in 2002, and Toyama University, Japan, in 2005, respectively. He joined the School of Computer Science and Technology at Shandong University as an associate professor in 2005, and joined the LAMDA group of Nanjing University, China, as a postdoctoral fellow in 2009. From 2010 to 2017, he was a professor at the School of Computer Science and Technology, Shandong University. He is the founder and the leader of MIMA (Machine Intelligence and Media Analysis) Lab of Shandong University. His research interests include machine learning, information retrieval, data mining and image/video analysis and retrieval. He has published in TIP, TKDE, TMM, TCSVT, AAAI, CIKM, IJCAI, MM, SIGIR, WWW and other venues. He also serves as an SPC/PC member or a reviewer for various international conferences and journals, e.g. AAAI, CIKM, CVPR, ICCV, IJCAI, MM, TCSVT, TIP, TKDE, TMM and TPAMI.
